# Supplementary material for: Neural 3D Reconstruction of Planetary Surfaces from Descent-Phase Wide-Angle Imagery
Source: arXiv:2604.13235 source file (2026-04-14)
Supplement: Supplementary file 1 [file X_suppl.tex]

\clearpage
\setcounter{page}{1}
\maketitlesupplementary

\section{Implementation and Resource details}

We developed our methodology on top of Nerfacto by Nerfstudio~\cite{nerfstudio2023}. We optimized our dual-pipeline on each dataset for 100K iterations and optimized Nerfacto baseline for 30K iterations on a local cluster running Ubuntu 22.04.1 with CUDA version 12.4. The cluster nodes are equipped with four NVIDIA A5000 GPUs (24GB VRAM each) and a single 16-core CPU with 128GB RAM. Each training run utilized a single GPU. 

Tuned hyperparameters for each dataset are listed below:

\begin{table}[h]
\centering
\caption{Hyperparameters for each dataset.}
\begin{tabular}{lcc}
\toprule
\textbf{Hyperparameter} & \textbf{Lunar} & \textbf{Mars} \\
\midrule
$t_{near}$ & 0.15 & 0.10 \\
$t_{far}$ & 500.0 & 10000.0 \\
$\lambda_{c;A}$ & 1.0 & 1.0 \\
$\lambda_{c;B}$ & 0.001 & 0.00001 \\
$\lambda_{height}$ $(it < 2000)$ & 0.0  & 0.0  \\
$\lambda_{height}$ $(2000 \leq it < 4000)$ & 1.0  & 1.0  \\
$\lambda_{height}$ $(it \geq 4000)$ & 0.001  & 0.001  \\
$\lambda_{dist}$ & 0.01 & 0.5 \\
${k_1}$ & 10000.0 & 10000.0 \\
${k_2}$ & 1000.0 & 1000.0 \\
\bottomrule
\end{tabular}
\label{tab:hyperparameters}
\end{table}
